# Supplementary material for: Scalable Application- and User-aware Resource Allocation in Enterprise Networks Using End-host Pacing
Source: arXiv:1811.02367 source file (2020-02-25)
Supplement: Supplementary file 1 [file 11_appendix_video.tex]

\section{Video Streaming Performance Details} \label{subsec:dash}

For video streaming we consider the two additional KPIs \textit{initial stalling time} and \textit{quality switching frequency}.
Initial stalling is the short unavoidable stalling time at the beginning of the video to download the first segment.
Stalling during the playback was prevented in all experiment runs by the quality adaptation algorithm.
Stallings and switches are not part of our utility functions $U_{VoD}$ and $U_{Live}$, but recent studies show their negative influence on the user's perceived video quality. \fixme{[][]}
Figures \ref{fig:23_dash_metrics} illustrate the median initial stalling time (\subref{fig:23_dash_metrics_stalling} and \subref{fig:23_dash_metrics_stalling_live}) and the median number of quality switches (\subref{fig:23_dash_metrics_switches} and \subref{fig:23_dash_metrics_switches_live}) per video view for \vod{} and \live{}.

In terms of initial stalling the figures show for the best effort case a strong linear correlation with the number of applications.
For \vod{}, the median stalling time increases approximately linear from \unit[0.9]{s} to \unit[4.5]{s} for 10 to 120 parallel applications.
For \live{}, the increase is from \unit[2.0]{s} to \unit[9.3]{s}.
%Hence, the quality adaption logic of the streaming clients is with increasing number of competing best effort flows less likely to achieve a continuous playback of the video.
%The fluctuating capacity and RTT make it difficult for the adaptation logic to estimate the available goodput.
In the managed case the initial stalling duration does not exceed \unit[1.9]{s} and \unit[5]{s} for \vod{} and \live{} up to $|A| < 100$, respectively.
For $|A| \geq 100$, the initial stalling increases to about \unit[10]{s}. 
This is due to fairness formulation assigning \live{} the minimum bandwidth which allows interruption-free playback of the video.
But with minimum bandwidth the initial buffer time increases.

%Hence, packet pacing and stable link QoS aid the adaptation logic in its decisions.

In terms of mean quality switches per playback minute, which is equal to the mean number of switches in the case of our \unit[60]{s} video, we observe a difference in behavior between \vod{} and \live{}.
For \vod{}, the switching frequency is low (approximately one or two switches per minute) for a small number of applications ($|A| \leq 30$) and for a large number of applications ($|A| > 110$).
In-between, the frequency ranges between \unit[1]{$m^{-1}$} and \unit[3]{$m^{-1}$} for the managed experiments and between \unit[2]{$m^{-1}$} and \unit[5]{$m^{-1}$} for the best effort experiments.
The reduced switching frequency for $|A| \leq 30$ and $|A| > 110$ can be explained by the fact that there are fewer reasonable choices for a quality level to choose when the goodput demand of the highest quality level is satisfied or the goodput demand for the lowest quality level is barely met.

For \live{}, the number of switches increases in the best effort experiments from 2.5 up to 6.5 switches and then decreases roughly linear to 0 for 120 applications.
As shown by Figure \ref{fig:21_per_app_std_model_video_live}, the utility, and therefor the mean quality level, drops fast to the lowest level with increasing number of applications for \live{} intent and best effort congestion control.
Hence, the number of switches for \live{} is also decreasing as the adaption logic has limited options and must often choose the lowest quality level.
In the managed case, the switches increase from \unit[2]{$m^{-1}$} to \unit[7]{$m^{-1}$} at 90 applications.
For $|A| \geq 100$ the switches drop to zero as only the lowest quality level is shown to the user.
The managed results show that the adaptation logic is not able to take advantage of the stable goodput for the \live{} intent.

In summary, data-rate management results in most cases in a smoother playback experience for the user in terms of quality switching.
There is also an opportunity for novel adaptation logics to further improve video adaptation.
If the bit-rate variations of all video chunks are known beforehand, which can be the case for DASH-based video streaming, a stable goodput allows for computing near-optimal adaptation decisions.

\begin{figure}[t]
\centering
\subfigure[Initial Stalling (\vod{})]{\includegraphics[width=105pt]{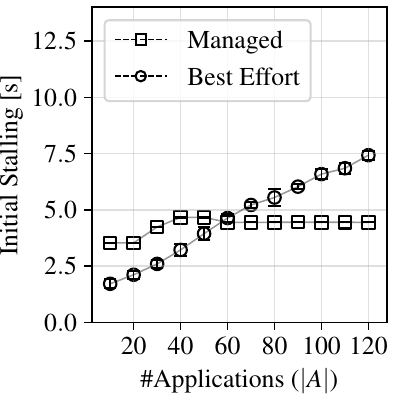}\label{fig:23_dash_metrics_stalling}}
\subfigure[Initial Stalling (\live{})]{\includegraphics[width=105pt]{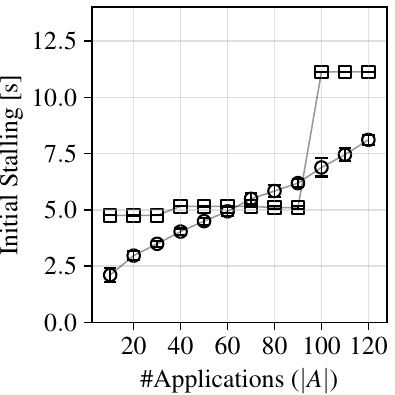}\label{fig:23_dash_metrics_stalling_live}}
\subfigure[Switches (\vod{})]{\includegraphics[width=105pt]{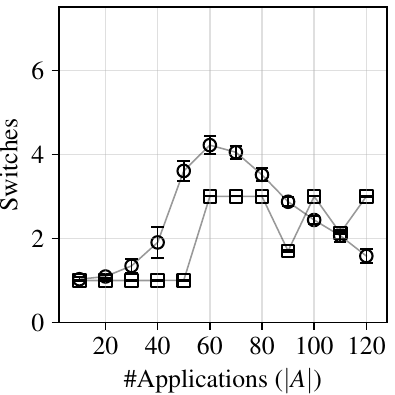}\label{fig:23_dash_metrics_switches}}
\subfigure[Switches (\live{})]{\includegraphics[width=105pt]{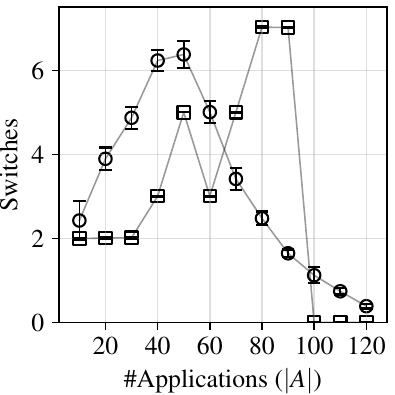}\label{fig:23_dash_metrics_switches_live}}\\
\caption{\textit{Initial stalling} duration and \textit{switching frequency} for the \vod{} and \live{} clients for increasing number of total applications.
There are no recorded stallings during the playback.}
\label{fig:23_dash_metrics}
\end{figure} 

% \subsection{Delay Bottleneck}
%\begin{figure}[h]
%\centering
%\subfigure[Delay]{\includegraphics[width=110pt]{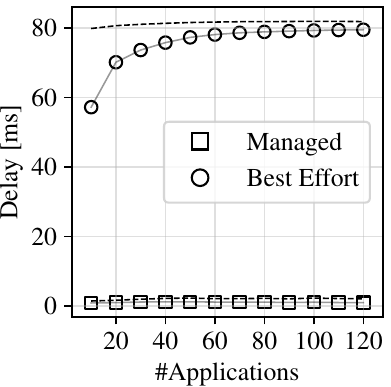}\label{fig:24_delay_delay}}
%\subfigure[std(Delay)]{\includegraphics[width=110pt]{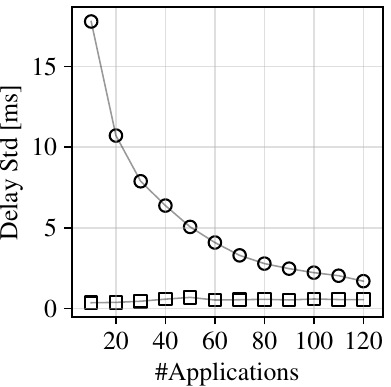}\label{fig:24_delay_std}}\\
%\caption{.....}
%\label{fig:23_dash_metrics}
%\end{figure} 
